# Supplementary material for: Operation of a Microfabricated Planar Ion-Trap for Studies of a Yb$^+$-Rb Hybrid Quantum System
Source: arXiv:1811.07670 source file (2019-03-19)
Supplement: Supplementary file 1 [file anleitung.tex]

%%
%% This is file `anleitung.tex',
%%
%% Copyright (C) 1994-2007 Axel Sommerfeldt (caption@sommerfee.de)
%% 
%% --------------------------------------------------------------------------
%% 
%% This work may be distributed and/or modified under the
%% conditions of the LaTeX Project Public License, either version 1.3
%% of this license or (at your option) any later version.
%% The latest version of this license is in
%%   http://www.latex-project.org/lppl.txt
%% and version 1.3 or later is part of all distributions of LaTeX
%% version 2003/12/01 or later.
%% 
%% This work has the LPPL maintenance status "maintained".
%% 
%% This Current Maintainer of this work is Axel Sommerfeldt.
%% 
%% This work consists of the files caption.ins, caption.dtx,
%% caption2.dtx, caption.xml, and anleitung.tex and the derived files
%% caption.sty, caption2.sty, caption3.sty, and manual.tex.
%% 
\ProvidesFile{anleitung.tex}
\NeedsTeXFormat{LaTeX2e}[1994/12/01]
\documentclass[a4paper]{ltxdoc}
\setlength\parindent{0pt}
\setlength\parskip{\medskipamount}

\errorcontextlines9
\def\StartTracing{\typeout{StartTracing}\tracingmacros=1\tracingcommands=1\relax}
\def\StopTracing{\tracingmacros=0\tracingcommands=0\relax\typeout{StopTracing}}

\newcommand\NEWfeature{\NEW{Neues Feature}}
\newcommand\NEWdescription{\NEW{Neue Beschreibung}}
\newcommand\NEW[2]{\hskip 1sp \marginpar{\footnotesize\sffamily\raggedleft#1\\#2}}

\font\manual=manfnt
\newcommand\DANGER{\hskip 1sp \marginpar{\raggedleft\textcolor{blue}{{\manual\char127}}}}

%%%\usepackage[T1]{fontenc}
\ifx\pdfoutput\undefined\else
  \ifcase\pdfoutput\else
    \usepackage{mathptmx,courier}
    \usepackage[scaled=0.90]{helvet}
    \addtolength\marginparwidth{15pt}
  \fi
\fi

\usepackage[german]{babel}
\usepackage{color,setspace}

%\usepackage{float}
\usepackage{longtable}
%\usepackage[raggedright]{sidecap}

\usepackage{caption}[2005/08/24]
\DeclareCaptionLabelSeparator{endash}{\space\textendash\space}
\usepackage{hyperref}

\DeclareCaptionFont{singlespacing}{\setstretch{1}}
\DeclareCaptionFont{onehalfspacing}{\onehalfspacing}
\DeclareCaptionFont{doublespacing}{\doublespacing}
\DeclareCaptionFont{red}{\color{red}}
\DeclareCaptionFont{green}{\color{green}}
\DeclareCaptionFont{blue}{\color{blue}}

\DeclareCaptionLabelSeparator{period-newline}{. \\}
\DeclareCaptionStyle{period-newline}[labelsep=period]{labelsep=period-newline}
\DeclareCaptionStyle{period-newline2}[labelsep=period,justification=centering]{labelsep=period-newline}
\DeclareCaptionStyle{period-newline3}[labelsep=period]{labelsep=period-newline,justification=centering}
\DeclareCaptionFormat{reverse}{#3#2#1}
\DeclareCaptionFormat{llap}{\llap{#1#2}#3\par}
\DeclareCaptionLabelFormat{fullparens}{(\bothIfFirst{#1}{ }#2)}
\DeclareCaptionLabelSeparator{fill}{\hfill}

\DeclareRobustCommand{\KOMAScript}{\textsf{K\kern.05em O\kern.05em%
    M\kern.05em A\kern.1em-\kern.1em Script}}

\newcommand*\purerm[1]{{\upshape\mdseries\rmfamily #1}}
\newcommand*\puresf[1]{{\upshape\mdseries\sffamily #1}}
\newcommand*\purett[1]{{\upshape\mdseries\ttfamily #1}}
\let\package\puresf\def\thispackage{\package{caption}}
\let\env\purett \let\opt\purett

\newcommand*\version[1]{$v#1$}

\newenvironment{Options}[1]%
  {\list{}{\renewcommand{\makelabel}[1]{\texttt{##1}\hfil}%
   \settowidth{\labelwidth}{\texttt{#1\space}}%
   \setlength{\leftmargin}{\labelwidth}%
   \addtolength{\leftmargin}{\labelsep}}}%
  {\endlist}

\newenvironment{Example}%
  {\ifvmode\else\unskip\par\fi
   \minipage{\linewidth}\smallskip}%
  {\smallskip\endminipage}
\newcommand\example[3][figure]{%
  \begingroup
    \captionsetup{#2}%
    \captionof{#1}[]{#3}%
  \endgroup}

\begin{document}

\GetFileInfo{caption.sty}
\title{Setzen von Abbildungs- und Tabellenbeschriftungen mit dem
       \thispackage-Paket\thanks{Dieses Paket hat die Versionsnummer
       \fileversion, zuletzt ge"andert am \filedate.}}
\author{Axel Sommerfeldt\\\href{mailto:caption@sommerfee.de}{\texttt{caption@sommerfee.de}}}
\date{9. April 2007}
\maketitle

\begin{abstract}
Das \thispackage\ Paket bietet einem Mittel und Wege das Erscheinungsbild der
Bildunterschriften und Tabellen"uberschriften den eigenen W"unschen
bzw.\ bestimmten Vorgaben anzupassen.
Hierbei wurde viel Wert auf die reibungslose Zusammenarbeit und in die
Integration anderer Dokumentenklassen und Pakete gelegt.\footnote{F"ur die
aktuelle Version 3.0 dieses Paketes wurde die Benutzerschnittstelle zusammen
mit Steven D. Cochran und Frank Mittelbach komplett "uberarbeitet.}
\end{abstract}

\tableofcontents

\newcommand\figuretext{%
  Die auf die Rotationsfrequenz des Innenzylinders normierten Eigenfrequenzen
  der gefundenen Grundmoden der Taylor"=Str"omung f"ur \mbox{$\eta = 0.5$}. %\\
  (Die azimutale Wellenzahl ist mit $m$ bezeichnet.)}

% --------------------------------------------------------------------------- %

\section{Einleitung}

Mit |\caption| gesetzte Bildunterschriften und Tabellen"uberschriften werden
von den Standard"=Dokumentenklassen eher stiefm"utterlich behandelt.
In der Regel schlicht als ganz normaler Absatz gesetzt, ergibt sich keine
signifikante optische Abgrenzung vom eigentlichen Text, wie z.B. hier:

\example{belowskip=\abovecaptionskip}{\figuretext}

Es sollte aber eine M"oglichkeit geben, diesem Umstand abzuhelfen. Es w"are
zum Beispiel nett, wenn man den Text der Unterschrift etwas kleiner gestalten,
extra R"ander festlegen oder den Zeichensatz des Bezeichners dem der
Kapitel"uberschriften anpassen k"onnte. So in etwa:

\example{belowskip=\abovecaptionskip,size=small,margin=10pt,labelfont=bf,labelsep=endash}{\figuretext}

Mit Hilfe dieses Paketes k"onnen Sie dies leicht bewerkstelligen; es sind viele
vorgegebene Parameter einstellbar, Sie k"onnen aber auch eigene
Gestaltungsmerkmale einflie"sen lassen.

% --------------------------------------------------------------------------- %

\pagebreak[4]
\section{Verwendung des Paketes}
\label{usage}

\DescribeMacro{\usepackage}
Mittels
\begin{quote}
  |\usepackage|\oarg{Optionen}|{caption}[|\texttt{\filedate}|]|
\end{quote}
in dem Vorspann des Dokumentes wird das \thispackage\ Paket eingebunden, die
Optionen legen hierbei das Aussehen der "Uber- und Unterschriften fest. So
w"urde z.B.
\begin{quote}
  |\usepackage[margin=10pt,font=small,labelfont=bf]{caption}|%[|\texttt{\filedate}|]|
\end{quote}
zu dem obrigen Ergebnis mit Rand, kleinerem Zeichensatz und fetter Bezeichnung
f"uhren.

\DescribeMacro{\captionsetup}
Eine "Anderung der Parameter ist auch zu einem sp"ateren Zeitpunkt jederzeit
mittels des Befehls
\begin{quote}
  |\captionsetup|\oarg{Typ}\marg{Optionen}
\end{quote}
m"oglich. So sind z.B. die Befehlssequenzen
\begin{quote}
  |\usepackage[margin=10pt,font=small,labelfont=bf]{caption}|%[|\texttt{\filedate}|]|
\end{quote}
und
\begin{quote}
  |\usepackage{caption}|\\%[|\texttt{\filedate}|]|
  |\captionsetup{margin=10pt,font=small,labelfont=bf}|
\end{quote}
in ihrer Wirkung identisch.

Weiterhin gilt zu beachten, da"s sich die Verwendung von |\captionsetup|
innerhalb von Umgebungen nur auf die Umgebung selber auswirkt, nicht aber auf
den Rest des Dokumentes. M"ochte man also z.B. die automatische Zentrierung der
Abbildungsunterschrift nur in einem konkreten Falle ausschalten, so kann dies
mit
\begin{quote}
  |\begin{figure}|\\
  |  |\ldots\\
  |  \captionsetup{singlelinecheck=off}|\\
  |  \caption{|\ldots|}|\\
  |\end{figure}|
\end{quote}
geschehen, ohne da"s die restlichen Abbildungsunterschriften hiervon
beeintr"achtigt werden.

(Der optionale Parameter \meta{Typ} wird in Abschnitt
 \ref{misc}: \textit{"`N"utzliches"'} behandelt.)

% --------------------------------------------------------------------------- %

\pagebreak[4]
\section{Beschreibung der Optionen}

\def\OptionLabel{RaggedRight}
\def\UserDefined{\ldots}
\makeatletter
\newcommand*\Section{\@ifstar{\@Section\relax}{\@Section{Abschnitt}}}
\newcommand*\@Section[3]{#1 \ref{#2}: \textit{"`#3"'}}
\makeatother
\newcommand*\See[1]{{\small (Siehe #1)}}
\newcommand*\SeeUserDefined[1][]{%
  \See{\Section{declare}{Eigene Erweiterungen}#1}}

% --------------------------------------------------------------------------- %

\subsection{Formatierung}

\DescribeMacro{format=}
Eine Abbildungs- oder Tabellenbeschriftung besteht im wesentlichen aus drei
Teilen:
Dem Bezeichner (etwa "`Abbildung 3"'), dem Trenner
(etwa "`:\textvisiblespace"') und dem eigentlichen Text.
Mittels der Option
\begin{quote}
  |format=|\meta{Name}
\end{quote}
wird festgelegt, wie diese drei Teile zusammengesetzt werden.
F"ur \meta{Name} sind folgende M"oglichkeiten verf"ugbar:%\footnote{Es gibt
%hier wie auch bei vielen anderen Optionen die M"oglichkeit, auch eigene
%Formate, Zeichens"atze etc.\ zu definieren. Wie dies geht wird in Abschnitt
%\ref{declare}: \textit{"`Eigene Erweiterungen"'} dargelegt.}

\begin{Options}{\OptionLabel}
  \item[plain]\NEWdescription{v3.0h}
  Die Beschriftung wird als gew"ohnlicher Abschnitt gesetzt.
  (Dies ist z.Z.~das Standardverhalten, ab Version $3.1$ des
   \package{caption} Paketes wird dies allerdings von der verwendeten
    Dokumentenklasse abh"angen.)

  \item[hang]
  Der Text wird so gesetzt, da"s er an dem Bezeichner "`h"angt"', d.h.~der
  Platz unter dem Bezeichner und dem Trenner bleibt leer.

  \item[\UserDefined]
  Eigene Formate k"onnen mittels |\DeclareCaptionFormat| definiert werden.
  \SeeUserDefined
\end{Options}

\begin{Example}
  Ein Beispiel: Die Angabe der Option
  \begin{quote}
    |format=hang|
  \end{quote}
  f"uhrt zu Abbildungsunterschriften der Art
  \example{format=hang}{\figuretext}
\end{Example}

\DescribeMacro{indention=}
Bei beiden Formaten (\texttt{plain} und \texttt{hang}) kann der Einzug der Beschriftung
ab der zweiten Textzeile angepasst werden, dies geschieht mit Hilfe der Option
\begin{quote}
  |indention=|\meta{Einzug}\quad,
\end{quote}
wobei anstelle von \meta{Einzug} jedes beliebige feste Ma"s angegeben werden kann.

Zwei Beispiele:

\begin{Example}
  \begin{quote}
    |format=plain,indention=.5cm|
  \end{quote}
  \captionsetup{aboveskip=0pt}
  \example{format=plain,indention=.5cm}{\figuretext}
\end{Example}

\begin{Example}
  \begin{quote}
    |format=hang,indention=-0.5cm|
  \end{quote}
  \captionsetup{aboveskip=0pt}
  \example{format=hang,indention=-0.5cm}{\figuretext}
\end{Example}

%\pagebreak[3]
\DescribeMacro{labelformat=}
Mittels der Option
\nopagebreak[3]
\begin{quote}
  |labelformat=|\meta{Name}
\end{quote}
\nopagebreak[3]
\NEWdescription{v3.0e}
wird die Zusammensetzung des Bezeichners festgelegt.
F"ur \meta{Name} sind folgende M"oglichkeiten verf"ugbar:

\begin{Options}{\OptionLabel}
  \item[default]
  Der Bezeichner wird wie von der verwendeten Dokumentenklasse vorgegeben gesetzt,
  "ublicherweise ist dies der Name und die Nummer, getrennt durch ein Leerzeichen
  (wie \texttt{simple}).
  (Dies ist das Standardverhalten.)

  \item[empty]
  Der Bezeichner ist leer. (Diese Option macht in der Regel nur in Verbindung mit
  anderen Optionen -- wie etwa \texttt{labelsep=none} -- Sinn.)

  \item[simple]
  Der Bezeichner ist aus dem Namen und der Nummer zusammengesetzt.

  \item[parens]
  Die Nummer des Bezeichners wird in runde Klammern gesetzt.

  \item[\UserDefined]
  Eigene Formate k"onnen mittels |\DeclareCaptionLabelFormat| definiert werden.
  \SeeUserDefined
\end{Options}

\begin{Example}
  Ein Beispiel: Die Optionen
  \begin{quote}
    |labelformat=parens,labelsep=quad|
  \end{quote}
  f"uhren zu Abbildungsunterschriften der Art
  \example{labelformat=parens,labelsep=quad}{\figuretext}
\end{Example}

\DescribeMacro{labelsep=}
Mittels der Option
\begin{quote}
  |labelsep=|\meta{Name}
\end{quote}
wird die Zusammensetzung des Trenners festgelegt.
F"ur \meta{Name} sind folgende M"oglichkeiten verf"ugbar:

\begin{Options}{\OptionLabel}
  \item[none]
  Der Trenner ist leer. (Diese Option macht in der Regel nur in Verbindung
  mit anderen Optionen -- wie etwa \texttt{labelformat=empty} -- Sinn.)

  \item[colon]
  Der Trenner besteht aus einem Doppelpunkt und einem Leerzeichen.
  (Dies ist z.Z.~das Standardverhalten.)

  \item[period]
  Der Trenner besteht aus einem Punkt und einem Leerzeichen.

  \item[space]
  Der Trenner besteht lediglich aus einem einzelnen Leerzeichen.

  \item[quad]
  Der Trenner besteht aus einem |\quad|.

  \item[newline]
  Als Trenner wird ein Zeilenumbruch verwendet.

  \item[endash]\NEWfeature{v3.0h}
  Als Trenner wird ein Gedankenstrich verwendet.

  \item[\UserDefined]
  Eigene Trenner k"onnen mittels |\DeclareCaptionLabelSeparator| definiert werden.
  \SeeUserDefined
\end{Options}

Drei Beispiele:
\begin{Example}
  \begin{quote}
    |labelsep=period|
  \end{quote}
  \captionsetup{aboveskip=0pt}
  \example{labelsep=period}{\figuretext}
\end{Example}

\begin{Example}
  \begin{quote}
    |labelsep=newline,singlelinecheck=false|
  \end{quote}
  \captionsetup{aboveskip=0pt}
  \example{labelsep=newline,singlelinecheck=false}{\figuretext}
\end{Example}

\begin{Example}
  \begin{quote}
    |labelsep=endash|
  \end{quote}
  \captionsetup{aboveskip=0pt}
  \example{labelsep=endash}{\figuretext}
\end{Example}

% --------------------------------------------------------------------------- %

\subsection{Textausrichtung}
\label{justification}

\DescribeMacro{justification=}
Mittels der Option
\begin{quote}
  |justification=|\meta{Name}
\end{quote}
wird die Ausrichtung des Textes festgelegt.
F"ur \meta{Name} sind folgende M"oglichkeiten verf"ugbar:

\begin{Options}{\OptionLabel}
  \item[justified]
  Der Text wird als Blocksatz gesetzt.
  (Dies ist z.Z.~das Standardverhalten.)

  \item[centering]
  Der Text wird zentriert gesetzt.

%  \item[Centering]
%  Der Text wird zentriert gesetzt. Hierf"ur wird jedoch im Gegensatz
%  zu \texttt{centering} der Befehl |\Centering| des \package{ragged2e}-Paketes
%  verwendet, der \LaTeX\ das Trennen der Worte erlaubt.

  \item[centerlast]
  Lediglich die letzte Zeile des Textes wird zentriert gesetzt.

  \item[centerfirst]
  Lediglich die erste Zeile des Textes wird zentriert gesetzt.

  \item[raggedright]
  Der Text wird linksb"undig gesetzt.

%  \item[RaggedRight]
%  Der Text wird linksb"undig mit Hilfe des \package{ragged2e}-Paketes gesetzt.
  \item[RaggedRight]
  Der Text wird ebenfalls linksb"undig gesetzt. Hierf"ur wird jedoch im Gegensatz
  zu \texttt{raggedright} der Befehl |\RaggedRight| des \package{ragged2e}-Paketes
  verwendet, der \LaTeX\ das Trennen der Worte erlaubt.

  \item[raggedleft]
  Der Text wird rechtsb"undig gesetzt.

%  \item[RaggedLeft]
%  Der Text wird rechtsb"undig mit Hilfe des \package{ragged2e}-Paketes gesetzt.

  \item[\UserDefined]
  Eigene Ausrichtungen k"onnen mittels |\DeclareCaptionJustification| definiert werden.
  \SeeUserDefined
\end{Options}

Einige Beispiele:
\begin{Example}
  \begin{quote}
    |justification=centerlast|
  \end{quote}
  \captionsetup{aboveskip=0pt}
  \example{justification=centerlast}{\figuretext}
\end{Example}

\begin{Example}
  \begin{quote}
    |format=hang,justification=raggedright|
  \end{quote}
  \captionsetup{aboveskip=0pt}
  \example{format=hang,justification=raggedright}{\figuretext}
\end{Example}

\begin{Example}
  \begin{quote}
    |format=hang,justification=RaggedRight|
  \end{quote}
  \captionsetup{aboveskip=0pt}
  \example{belowskip=\abovecaptionskip,format=hang,justification=RaggedRight}{\figuretext}
\end{Example}

\begin{Example}
  \begin{quote}
    |labelsep=newline,justification=centering|
  \end{quote}
  \captionsetup{aboveskip=0pt}
  \example{belowskip=\abovecaptionskip,labelsep=newline,justification=centering}{\figuretext}
\end{Example}

\DescribeMacro{singlelinecheck=}
In den Standard"=Dokumentenclassen |article|, |report| und |book| sind die
Ab\-bildungs- und Tabellenbeschriftungen so realisiert, da"s sie automatisch
zentriert werden, wenn sie lediglich aus einer einzigen Textzeile bestehen:

\example{belowskip=\abovecaptionskip}{Eine kurze Beschriftung.}

%\example{belowskip=\abovecaptionskip}{%
% Eine lange Beschriftung, die gen"ugend Text enth"alt, um l"anger als
% eine einzelne Zeile zu sein.}

\DANGER
Diesen Mechanismus "ubernimmt das \thispackage-Paket und ignoriert damit
in der Regel bei solch kurzen Beschriftungen die mittels der Option
|justification=| eingestellte Textausrichtung. Dieses Verhalten kann
jedoch mit der Option
\begin{quote}
  |singlelinecheck=|\meta{bool}
\end{quote}
reguliert werden. Setzt man f"ur \meta{bool} entweder |false|, |no|, |off|
oder |0| ein, so wird der Zentrierungsmechnismus au"ser Kraft gesetzt.
Die obrige, kurze Abbildungsunterschrift w"urde z.B. nach Angabe der Option
\begin{quote}
  |singlelinecheck=false|
\end{quote}
so aussehen:
\begingroup
\captionsetup{type=figure}
\ContinuedFloat
\endgroup
\example{belowskip=\abovecaptionskip,singlelinecheck=false}{Eine kurze Beschriftung.}

Setzt man f"ur \meta{bool} hingegen |true|, |yes|, |on| oder |1| ein, so
wird die automatische Zentrierung wieder eingeschaltet. (Standardm"a"sig
ist sie eingeschaltet.)

% --------------------------------------------------------------------------- %

\subsection{Zeichens"atze}

\DescribeMacro{font=}
\DescribeMacro{labelfont=}
\DescribeMacro{textfont=}
Das \thispackage-Paket kennt 3 Zeichens"atze: Denjenigen f"ur die gesammte Beschriftung
(|font|), denjenigen, der lediglich auf den Bezeichner und den Trenner angewandt wird
(|labelfont|), sowie denjenigen, der lediglich auf den Text wirkt (|textfont|).
So lassen sich die unterschiedlichen Teile der Beschriftung individuell mittels
\begin{quote}\begin{tabular}{@{}r@{}ll}
  |font=|      & \marg{Zeichensatzoptionen} & ,\\
  |labelfont=| & \marg{Zeichensatzoptionen} & und\\
  |textfont=|  & \marg{Zeichensatzoptionen} & \\
\end{tabular}\end{quote}
\nopagebreak[3]
anpassen.
\pagebreak[3]

Als \meta{Zeichensatzoptionen} sind eine Kombination aus folgendem erlaubt:

\begin{Options}{\OptionLabel}
  \item[scriptsize]   {\scriptsize Sehr kleine Schrift}
  \item[footnotesize] {\footnotesize Fu"snotengr"o"se}
  \item[small]        {\small Kleine Schrift}
  \item[normalsize]   {\normalsize Normalgro"se Schrift}
  \item[large]        {\large Gro"se Schrift}
  \item[Large]        {\Large Gr"o"sere Schrift}

  \item[up]           {\upshape Upright Schriftart}
  \item[it]           {\itshape Italic Schriftart}
  \item[sl]           {\slshape Slanted Schriftart}
  \item[sc]           {\scshape Small Caps Schriftart}

  \item[md]           {\mdseries Medium Schriftserie}
  \item[bf]           {\bfseries Bold Schriftserie}

  \item[rm]           {\rmfamily Roman Schriftfamilie}
  \item[sf]           {\sffamily Sans Serif Schriftfamilie}
  \item[tt]           {\ttfamily Typewriter Schriftfamilie}

  \item[\UserDefined]
  Eigene Zeichensatzoptionen k"onnen mittels |\DeclareCaptionFont| definiert werden.
  \SeeUserDefined
\end{Options}

Wird lediglich eine einzelne Zeichensatzoption ausgew"ahlt, k"onnen die
geschweiften Klammern entfallen, d.h.~die Optionen
%\begin{quote}
  |font={small}|
%\end{quote}
und
%\begin{quote}
  |font=small|
%\end{quote}
sind in ihrer Wirkung identisch.

Beispiele:
\begin{Example}
  \begin{quote}
    |font={small,it},labelfont=bf|
  \end{quote}
  \captionsetup{aboveskip=0pt}
  \example{font={small,it},labelfont=bf}{\figuretext}
\end{Example}

\begin{Example}
  \begin{quote}
    |font=small,labelfont=bf,textfont=it|
  \end{quote}
  \captionsetup{aboveskip=0pt}
  \example{font=small,labelfont=bf,textfont=it}{\figuretext}
\end{Example}

% --------------------------------------------------------------------------- %

\subsection{R"ander und Abs"atze}
\label{margins}

\DescribeMacro{margin=}
\DescribeMacro{width=}
F"ur die Abbildungs- und Tabellenbeschriftungen kann \emph{entweder} ein extra Rand
\emph{oder} eine feste Breite festgelegt werden. Dies geschieht mit
\begin{quote}\begin{tabular}{@{}r@{}ll}
  |margin=| & \meta{Rand} & \emph{oder}\\
  |width=|  & \meta{Breite} & \\
\end{tabular}\end{quote}
In beiden F"allen wird die Beschriftung zentriert, d.h.~der linke und rechte Rand
sind immer gleich gro"s.

Zwei Beispiele hierzu:
\begin{Example}
  \begin{quote}
    |margin=10pt|
  \end{quote}
  \captionsetup{aboveskip=0pt}
  \example{margin=10pt}{\figuretext}
\end{Example}

\begin{Example}
  \begin{quote}
    |width=.75\textwidth|
  \end{quote}
  \captionsetup{aboveskip=0pt}
  \example{width=.75\textwidth}{\figuretext}
\end{Example}

\DescribeMacro{parskip=}
Diese Option wirkt auf Abbildungs- oder Tabellenbeschriftungen, die
aus mehr als einem Absatz bestehen; sie legt den Abstand zwischen den
Abs"atzen fest.
\begin{quote}
  |parskip=|\meta{Abstand zwischen Abs"atzen}
\end{quote}
Ein Beispiel:
\begin{Example}
  \begin{quote}
    |margin=10pt,parskip=5pt|
  \end{quote}
  \captionsetup{aboveskip=0pt}
  \example{margin=10pt,parskip=5pt}{%
    Erster Absatz der Beschriftung; dieser enth"alt einigen Text, so da"s die
    Auswirkungen der Optionen deutlich werden.

    Zweiter Absatz der Beschriftung; dieser enth"alt ebenfalls einigen Text,
    so da"s die Auswirkungen der Optionen deutlich werden.}
\end{Example}

\DescribeMacro{hangindent=}
Die Option
\begin{quote}
  |hangindent=|\meta{Einzug}
\end{quote}
legt einen Einzug f"ur alle Zeilen au"ser der jeweils ersten des Absatzes fest.
Besteht die Beschriftung lediglich aus einem einzelnen Absatz, so ist die
Wirkung mit der Option |indention=|\meta{Einzug} identisch, bei mehreren
Abs"atzen zeigt sich jedoch der Unterschied:

\begin{Example}
  \begin{quote}
    |format=hang,indention=-.5cm|
  \end{quote}
  \captionsetup{aboveskip=0pt}
  \example{format=hang,indention=-.5cm}{%
    Erster Absatz der Beschriftung; dieser enth"alt einigen Text, so da"s die
    Auswirkungen der Optionen deutlich werden.

    Zweiter Absatz der Beschriftung; dieser enth"alt ebenfalls einigen Text,
    so da"s die Auswirkungen der Optionen deutlich werden.}
\end{Example}

\begin{Example}
  \begin{quote}
    |format=hang,hangindent=-.5cm|
  \end{quote}
  \captionsetup{aboveskip=0pt}
  \example{format=hang,hangindent=-.5cm}{%
    Erster Absatz der Beschriftung; dieser enth"alt einigen Text, so da"s die
    Auswirkungen der Optionen deutlich werden.

    Zweiter Absatz der Beschriftung; dieser enth"alt ebenfalls einigen Text,
    so da"s die Auswirkungen der Optionen deutlich werden.}
\end{Example}

% --------------------------------------------------------------------------- %

\subsection{Stile}
\label{style}

\DescribeMacro{style=}
Eine geeignete Kombination aus den bisher vorgestellten Optionen wird \textit{Stil}
genannt; dies ist in etwa mit dem Seitenstil vergleichbar, den man bekannterma"sen
mit |\pagestyle| einstellen kann.

Einen vordefinierten Abbildungs- und Tabellenbeschriftungsstil kann man mit der
Option
\begin{quote}
  |style=|\meta{Stil}
\end{quote}
ausw"ahlen. Das \thispackage-Paket definiert in der Regel lediglich den Stil
|default|, der alle vorgehenden Optionen auf die Standardbelegung zur"ucksetzt,
d.h.~die Angabe der Option
\begin{quote}
  |style=default|
\end{quote}
entspricht den Optionen
\begin{quote}
  |format=default,labelformat=default,labelsep=default,|\\
  |justification=default,font=default,labelfont=default,|\\
  |textfont=default,margin=0pt,indention=0pt,parindent=0pt|\\
  |hangindent=0pt,singlelinecheck=true|
\end{quote}

Eigene Stile k"onnen mittels |\DeclareCaptionStyle| definiert werden.
\SeeUserDefined


% --------------------------------------------------------------------------- %

\subsection{Abst"ande}

\DescribeMacro{aboveskip=}
\DescribeMacro{belowskip=}
Die Standard-\LaTeX-Klassen |article|, |report| und |book| definieren
zwei Abst"ande, die in Zusammenhang mit den Abbildungs- und
Tabellenbeschriftungen gebraucht werden: |\abovecaptionskip| wird \emph{vor}
der Beschriftung angewandt und ist auf |10pt| vorbelegt. |\belowcaptionskip|
wird \emph{nach} der Beschriftung angewandt und ist auf |0pt| vorbelegt.

\pagebreak[3]
Beide Abst"ande lassen sich gew"ohnlich mit |\setlength| "andern, aber auch mit den
\thispackage-Optionen
\nopagebreak[3]
\begin{quote}\begin{tabular}{@{}r@{}ll}
  |aboveskip=| & \meta{Abstand nach oben}  & und\\
  |belowskip=| & \meta{Abstand nach unten} & .\\
\end{tabular}\end{quote}

\DescribeMacro{position=}
Die sture Anwendung von |\abovecaptionskip| und |\belowcaptionskip| bei
Beschriftungen birgt einen gro"sen Nachteil: Ist die Beschriftung \emph{"uber}
und nicht \emph{unter} der Abbildung oder Tabelle (wie bei Tabellen durchaus
"ublich), so ist die Vorbelegung dieser beiden Abst"ande nicht mehr sinnvoll,
da hier kein Abstand zwischen der Beschriftung und der Tabelle gesetzt wird.
(Wir erinnern uns: |\belowcaptionskip| ist auf |0pt|, also kein Abstand,
vorbelegt.)

Man vergleiche:
\begin{Example}
  \begin{minipage}[c]{.5\linewidth}%
%   \captionsetup{aboveskip=0pt}%
    \captionof{table}{Eine Tabelle}%
    \centering\begin{tabular}{ll}%
      A & B \\%
      C & D \\%
    \end{tabular}%
  \end{minipage}%
  \begin{minipage}[c]{.5\linewidth}%
    \centering\begin{tabular}{ll}%
      A & B \\%
      C & D \\%
    \end{tabular}%
    \captionof{table}{Eine Tabelle}%
  \end{minipage}%
\end{Example}

Mit Hilfe des Parameters |position| kann man jedoch festlegen, wie
\LaTeX\ die Beschriftung behandeln soll, ob als \mbox{\emph{"Uber}schrift}
oder als \mbox{\emph{Unter}schrift}:
\begin{quote}
  |position=top|\quad(oder |position=above|)
\end{quote}
gibt an, da"s die Abst"ande so gew"ahlt werden, da"s sie f"ur \mbox{\emph{"Uber}schriften}
sinnvoll gew"ahlt sind und
\begin{quote}
  |position=bottom|\quad(oder |position=below|)
\end{quote}
gibt an, da"s die Abst"ande so gew"ahlt werden, da"s sie f"ur \mbox{\emph{"Uber}schriften}
sinnvoll gew"ahlt sind. (Dies ist die Standardeinstellung, allerdings nicht f"ur |longtable|s.)

F"ugt man nun ein |\captionsetup{position=top}| in die linke Tabelle vor dem
|\caption| Befehl ein, so ergeben sich im Vergleich zwischen "Uberschrift und
Unterschrift stimmige Abst"ande:
\begin{Example}
  \begin{minipage}[c]{.5\linewidth}%
    \captionsetup{position=top}%
    \captionof{table}{Eine Tabelle}%
    \centering\begin{tabular}{ll}%
      A & B \\%
      C & D \\%
    \end{tabular}%
  \end{minipage}%
  \begin{minipage}[c]{.5\linewidth}%
    \centering\begin{tabular}{ll}%
      A & B \\%
      C & D \\%
    \end{tabular}%
    \captionof{table}{Eine Tabelle}%
  \end{minipage}%
\end{Example}

(Technisch ist dies so realisiert, da"s bei "Uberschriften die Ab\-st"an\-de
|\abovecaptionskip| und |\belowcaptionskip| vertauscht werden, so da"s
|\abovecaptionskip| immer derjenige Abstand ist, der zwischen Tabelle
und Beschriftung zur Anwendung kommt.)

Sinnvoll l"a"st sich diese Option insbesondere zusammen mit dem optionalen
Parameter bei |\captionsetup| anwenden: \See{auch \Section{misc}{N"utzliches}}
\begin{quote}
  |\captionsetup[table]{position=top}|
\end{quote}
bewirkt, da"s bei allen Tabellen die Beschriftung bzgl.~der Abst"ande als
"Uberschrift behandelt wird.
\DescribeMacro{tableposition=}
\NEWfeature{v3.0a}
Da dies eine sehr gebr"auchliche Einstellung ist,
stellt das \thispackage"=Paket diesen Befehl auch als abk"urzende Option f"ur
|\usepackage| zur Verf"ugung:
\begin{quote}
  |\usepackage[|\ldots|,tableposition=top]{caption}|\footnote{Beachten
  Sie bitte, da"s dies \emph{nicht} ausreichend ist, wenn eine
  \KOMAScript\ Dokumentenklasse zum Einsatz kommt. In diesem Falle mu"s
  ebenfalls die \emph{globale} Option |tablecaptionabove| angegeben werden.}
\end{quote}
entspricht
\begin{quote}
  |\usepackage[|\ldots|]{caption}|\\
  |\captionsetup[table]{position=top}|
\end{quote}

% --------------------------------------------------------------------------- %

\pagebreak[3]
\section{N"utzliches}
\label{misc}

\DescribeMacro{\caption}
Der Befehl
\nopagebreak[3]
\begin{quote}
  |\caption|\oarg{Kurzform f"ur das Verzeichnis}\marg{Beschriftung}
\end{quote}
\nopagebreak[3]
erzeugt eine "Uber- bzw.~Unterschrift innerhalb einer gleitenden Umgebung
wie |figure| oder |table|. Dies ist an sich nichts neues, neu ist allerdings,
da"s kein Eintrag ins Abbildungs- oder Tabellenverzeichnis vorgenommen
wird, wenn eine leere Kurzform angegeben wird, etwa so:
\begin{quote}
  |\caption[]{Dies ist eine Abbildung, die nicht ins|\\
  |           Abbildungsverzeichnis aufgenommen wird}|
\end{quote}

\DescribeMacro{\caption*}
Das \package{longtable}-Paket definiert zus"atzlich zum Befehl |\caption| auch
den Befehl |\caption*|, der eine Beschriftung ohne Bezeichner und ohne Eintrag
ins Tabellenverzeichnis erzeugt. So erzeugt z.B. der Code
\begin{quote}
  |\begin{longtable}{cc}|\\
  |  \caption*{Eine Tabelle}\\|\\
  |  A & B \\|\\
  |  C & D \\|\\
  |\end{longtable}|
\end{quote}
diese Tabelle:
\begin{longtable}{cc}
  \caption*{Eine Tabelle}\\
  A & B \\
  C & D \\
\end{longtable}

Das \thispackage-Paket bietet diesen Mechanismus auch f"ur normale Abbildungs-
und Tabellenbeschriftungen an. Ein Beispiel:
\begin{quote}
  |\begin{table}|\\
  |  \caption*{Eine Tabelle}|\\
  |  \begin{tabular}{cc}|\\
  |    A & B \\|\\
  |    C & D \\|\\
  |  \end{tabular}|\\
  |\end{table}|
\end{quote}

\DescribeMacro{\captionof}
\DescribeMacro{\captionof*}
Der Befehl |\caption| funktioniert in der Regel nur innerhalb von gleitenden
Umgebungen, manchmal m"ochte man ihn jedoch auch anderweitig anwenden,
etwa um eine Abbildung in eine nicht-gleitende Umgebung wie |minipage| zu
setzen.

\pagebreak[2]
Hierf"ur stellt das
\thispackage-Paket den Befehl
\begin{quote}
  |\captionof|\marg{Umgebungstyp}\oarg{Kurzform}\marg{Langform}
\end{quote}
zur Verf"ugung. Die Angabe des Umgebungstypen ist hierbei notwendig, damit der
gew"unschte Bezeichner gew"ahlt wird und der Eintrag in das richtige Verzeichnis
vorgenommen wird. Ein Beispiel:
\begin{quote}
  |\captionof{figure}{Abbildung}|\\
  |\captionof{table}{Tabelle}|
\end{quote}
f"uhrt zu folgendem Ergebnis:
\begin{Example}
  \captionof{figure}{Abbildung}
  \captionsetup{belowskip=\abovecaptionskip}
  \captionof{table}{Tabelle}
\end{Example}

Analog zu |\caption*| gibt es auch den Befehl |\captionof*| f"ur Beschriftungen
ohne Bezeichner und ohne Verzeichniseintrag.

Beide Befehle, sowohl |\captionof| als auch |\captionof*|, sollten nur
\emph{innerhalb} von Umgebungen (wie |minipage| oder |\parbox|) angewandt werden.
Zum einen kann es sonst passieren, da"s \LaTeX\ zwischen dem Inhalt und der
Beschreibung einen Seitenumbruch setzt; zum anderen kann es bei Mi"sachtung gar
zu seltsamen Effekten (wie falsche Abst"ande um die Beschriftungen herum) kommen!

\DescribeMacro{\ContinuedFloat}
Manchmal m"ochte man Abbildungen oder Tabellen aufteilen, jedoch ohne den einzelnen
Teilen eine eigene Abbildungs- oder Tabellennummer zu geben. Hierf"ur stellt das
\thispackage-Paket den Befehl
\begin{quote}
  |\ContinuedFloat|
\end{quote}
zur Verf"ugung, der gleich als erstes innerhalb der folgenden Teile angewandt
werden sollte. Er verhindert, da"s die Z"ahlung fortgef"uhrt wird; eine Abbildung
oder Tabelle, die ein |\ContinuedFloat| enth"alt, erh"alt also die gleiche Nummer
wie die vorherige Abbildung oder Tabelle.

Ein Beispiel:
\begin{quote}
  |\begin{table}|\\
  |\caption{Eine Tabelle.}|\\
  \ldots\\
  |\end{table}|\\
  \ldots\\
  |\begin{table}\ContinuedFloat|\\
  |\caption{Eine Tabelle. (fortgef"uhrt)}|\\
  \ldots\\
  |\end{table}|
\end{quote}
ergibt als Ergebnis:
\begin{Example}
  \makeatletter\def\@captype{table}\makeatother
  \caption[]{Eine Tabelle.}
  \centerline{\ldots}
  \ContinuedFloat
  \captionsetup{aboveskip=0pt}
  \caption[]{Eine Tabelle. (fortgef"uhrt)}
\end{Example}

\DescribeMacro{\captionsetup}
Den Befehl |\captionsetup| haben wir ja schon im \Section{usage}
{Verwendung des Paketes} kennengelernt,
uns dort allerdings die Bedeutung des optionalen Parameters
\meta{Typ} aufgespart. %Dies soll nun nachgeholt werden:

Wir erinnern uns, die Syntax des Befehls lautet
\begin{quote}
  |\captionsetup|\oarg{Typ}\marg{Optionen}
\end{quote}

Wird hierbei ein \meta{Typ} angegeben, so werden die Optionen nicht
unmittelbar umgesetzt, sondern werden lediglich vermerkt und kommen erst dann
zum Einsatz, wenn eine "Uber- bzw.\ Unterschrift innerhalb des passenden
gleitenden Umgebungstyps gesetzt wird. So wirkt sich z.B. die Angabe
\begin{quote}
  |\captionsetup[figure]|\marg{Optionen}
\end{quote}
lediglich auf die Unterschriften aus, die innerhalb einer |figure|"=Umgebung
gesetzt werden.

Ein Beispiel:
\begin{quote}
  |\captionsetup{font=small}|\\
  |\captionsetup[figure]{labelfont=bf}|
\end{quote}
f"uhrt zu Abbildungs- und Tabellenunterschriften der Art:
\begin{Example}
  \captionsetup{font=small}
  \captionsetup[figure]{labelfont=bf}
  \captionof{figure}[]{Eine Abbildung}
  \captionsetup{belowskip=\abovecaptionskip}
  \captionof{table}[]{Eine Tabelle}
\end{Example}

Wie man sieht, f"uhrt das |\captionsetup[figure]{labelfont=bf}| lediglich dazu,
da"s Abbildungsunterschriften mit fettem Bezeichner gesetzt werden, alle anderen
Unter- bzw.\ "Uberschriften werden hiervon nicht beeinflu"st.

\DescribeMacro{\clearcaptionsetup}
Um diese vermerkten, typbezogenen Parameter aus dem Ged"achnis von \LaTeX\ zu
l"oschen, gibt es den Befehl
\begin{quote}
  |\clearcaptionsetup|\marg{Typ}\quad.
\end{quote}

|\clearcaptionsetup{figure}| w"urde z.B. die obrige Sonderbehandlung der
Abbildungsunterschriften wieder aufheben:
\begin{Example}
  \captionsetup{font=small}
   \captionof{figure}[]{Eine Abbildung}
   \captionsetup{belowskip=\abovecaptionskip}
   \captionof{table}[]{Eine Tabelle}
\end{Example}

Als Umgebungstypen mit Unter- bzw.\ "Uberschriften gibt es in der Regel nur
zwei: |figure| und |table|. Wie wir jedoch sp"ater sehen werden, kommen durch die
Verwendung spezieller \LaTeX-Pakete (wie etwa das \package{float},
\package{longtable} oder \package{sidecap}"=Paket)
ggf.~weitere Typen hinzu, deren Beschriftungen ebenfalls derart individuell
angepasst werden k"onnen.

% --------------------------------------------------------------------------- %

\pagebreak[4]
\section{Eigene Erweiterungen}
\label{declare}

Wem die vorhandenen Formate, Trenner, Textausrichtungen, Zeichens"atze und Stile
nicht ausreichen, der hat die M"oglichkeit, sich eigene zu definieren. Hierzu
gibt es eine Reihe von Befehlen, die in dem Vorspann des Dokumentes (das ist der
Teil vor |\begin{document}|) zum Einsatz kommen.

\pagebreak[2]
\DescribeMacro{\DeclareCaptionFormat}
Eigene Formate k"onnen mit dem Befehl
\begin{quote}
  |\DeclareCaptionFormat|\marg{Name}\marg{Code mit \#1, \#2 und \#3}
\end{quote}
definiert werden. F"ur \#1 wird sp"ater der Bezeichner, f"ur \#2 der Trenner
und f"ur \#3 der Text eingesetzt. So ist z.B. das Standardformat |plain|,
welches die Beschriftung als gew"ohnlichen Absatz formatiert, folgenderma"sen
in |caption.sty| definiert:
\begin{quote}
  |\DeclareCaptionFormat{plain}{#1#2#3\par}|
\end{quote}

\DescribeMacro{\DeclareCaptionLabelFormat}
"Ahnlich k"onnen auch eigene Bezeichnerformate definiert werden:
\begin{quote}
  |\DeclareCaptionLabelFormat|\marg{Name}\marg{Code mit \#1 und \#2}
\end{quote}
Bei den Bezeichnerformaten wird hierbei f"ur \#1 der Name (also z.B.
"`Abbildung"'), f"ur \#2 die Nummer (also z.B. "`12"') eingesetzt.

\DescribeMacro{\bothIfFirst}
\DescribeMacro{\bothIfSecond}
Hierbei gibt es eine Besonderheit zu beachten: Wird das Bezeichnerformat
auch in Verbindung mit dem \package{subfig}"=Paket\cite{subfig} verwendet,
so kann der Bezeichnername (also \#1) auch leer sein.
Um dies flexibel handhaben zu k"onnen, stellt das \thispackage"=Paket die
Befehle
\begin{quote}
  |\bothIfFirst|\marg{Erstes Argument}\marg{Zweites Argument}\quad und\\
  |\bothIfSecond|\marg{Erstes Argument}\marg{Zweites Argument}
\end{quote}
zur Verf"ugung. |\bothIfFirst| testet, ob das erste Argument leer ist,
|\bothIfSecond|, ob das zweite Argument leer ist. Nur wenn dies nicht der
Fall ist, werden beide Argumente ausgegeben, ansonsten werden beide
unterdr"uckt.

So ist z.B. das Standard"=Bezeichnerformat |simple| nicht, wie man
naiverweise annehmen k"onnte, als
\begin{quote}
  |\DeclareCaptionLabelFormat{simple}{#1 #2}|
\end{quote}
definiert, weil dies zu einem st"orendem f"uhrenden Leerzeichen f"uhren w"urde,
wenn \#1 leer ist. Stattdessen findet sich in |caption.sty| folgende
Definition, die sowohl mit |\caption| als auch mit |\subfloat| harmoniert:
\begin{quote}
  |\DeclareCaptionLabelFormat{simple}{\bothIfFirst{#1}{ }#2}|
\end{quote}
d.h.~das Leerzeichen kommt nur dann zum Einsatz, wenn \#1 nicht leer ist.

\pagebreak[3]
\DescribeMacro{\DeclareCaptionLabelSeparator}
Eigene Trenner werden mit
\nopagebreak[3]
\begin{quote}
  |\DeclareCaptionLabelSeparator|\marg{Name}\marg{Code}
\end{quote}
\nopagebreak[3]
definiert. Auch hier wieder als einfaches Beispiel die Definition des
Standard"=Trenners aus |caption.sty|:
\nopagebreak[3]
\begin{quote}
  |\DeclareCaptionLabelSeparator{colon}{: }|
\end{quote}
\pagebreak[3]

\DescribeMacro{\DeclareCaptionJustification}
Eigene Textausrichtungen k"onnen mit
\begin{quote}
  |\DeclareCaptionJustification|\marg{Name}\marg{Code}
\end{quote}
definiert werden. Der \meta{Code} wird dann der Beschriftung vorangestellt,
so f"uhrt z.B. die Verwendung der Ausrichtung
\begin{quote}
  |\DeclareCaptionJustification{raggedright}{\raggedright}|
\end{quote}
dazu, da"s alle Zeilen der Beschriftung linksb"undig ausgegeben werden.

\DescribeMacro{\DeclareCaptionFont}
Eigene Zeichensatzoptionen k"onnen mit
\begin{quote}
  |\DeclareCaptionFont|\marg{Name}\marg{Code}
\end{quote}
definiert werden. So definiert z.B. das \thispackage"=Paket die Optionen
|small| und |bf| folgenderma"sen:
\begin{quote}
  |\DeclareCaptionFont{small}{\small}|\\
  |\DeclareCaptionFont{bf}{\bfseries}|
\end{quote}
Die Zeilenabst"ande lie"sen sich z.B.~"uber das \package{setspace}"=Paket
regeln:\NEWdescription{v3.0h}
\begin{quote}
  |\usepackage{setspace}|\\
\iffalse
  |\DeclareCaptionFont{singlespacing}{\setstretch{1}}|\quad\footnote{%
  \emph{Hinweis:} \cs{singlespacing} kann hier nicht benutzt werden, da es ein \cs{vskip} Kommando enth"alt.}\\
  |\DeclareCaptionFont{onehalfspacing}{\onehalfspacing}|\\
  |\DeclareCaptionFont{doublespacing}{\doublespacing}|\\
\fi
  |\captionsetup{font={onehalfspacing,small},labelfont=bf}|
\end{quote}
\example{font={onehalfspacing,small},labelfont=bf,singlelinecheck=off}\figuretext
Ein Beispiel welches etwas Farbe ins Spiel bringt:
\begin{quote}
  |\usepackage{color}|\\
  |\DeclareCaptionFont{red}{\color{red}}|\\
  |\DeclareCaptionFont{green}{\color{green}}|\\
  |\DeclareCaptionFont{blue}{\color{blue}}|\\
  |\captionsetup{labelfont=blue,textfont=green}|
\end{quote}
\example{labelfont=blue,textfont=green,singlelinecheck=off}\figuretext

\DescribeMacro{\DeclareCaptionStyle}
Zu guter letzt noch die Definition eigener Stile. Stile sind einfach eine
Ansammlung von geeigneten Einstellungen, die unter einem eigenen Namen
zusammengefasst werden und mit der Paketoption |style=|\meta{Name} ausgew"ahlt
werden k"onnen. Sie werden wie folgt definiert:
\begin{quote}
  |\DeclareCaptionStyle|\marg{Name}\oarg{zus"atzliche Optionen}\marg{Optionen}
\end{quote}
Hierbei ist zu beachten, da"s die \meta{Optionen} immer auf den Standardeinstellungen
basieren (siehe auch \Section{style}{Stile}), es brauchen
also nur davon abweichende Optionen angegeben werden.

Sind \meta{zus"atzliche Optionen} angegeben, so kommen diese automatisch
zus"atzlich zum Einsatz, sofern die Beschreibung in eine einzelne Zeile passt
und diese Abfrage nicht mit |singlelinecheck=off| ausgeschaltet wurde.

Als Beispiel mu"s mal wieder eine einfache Definition aus diesem Paket herhalten:
\begin{quote}
  |\DeclareCaptionStyle{default}[justification=centering]{}|
\end{quote}

% --------------------------------------------------------------------------- %

\subsection{Weiterf"uhrende Beispiele}

M"ochte man als Trenner einen Punkt \emph{und} einen Zeilenumbruch haben,
so lie"se sich das wie folgt realisieren:
\begin{quote}
  |\DeclareCaptionLabelSeparator{period-newline}{. \\}|
\end{quote}
W"ahlt man diesen Trenner mit |\captionsetup{labelsep=period-newline}| aus, so
ergeben sich Beschriftungen der Art
\begin{Example}
  \captionsetup{labelsep=period-newline,labelfont=bf,margin=10pt}
  \captionsetup{aboveskip=0pt,type=figure}
  \caption[]{\figuretext}
\end{Example}

F"ur kurze Beschriftungen, die in eine Zeile passen, mag dieses Erscheinungsbild
jedoch st"orend sein, selbst wenn die automatische Zentrierung (mit
|singlelinecheck=off|) ausgeschaltet ist:
\begin{Example}
  \captionsetup{labelsep=period-newline,labelfont=bf,margin=10pt,singlelinecheck=0}
  \captionsetup{aboveskip=0pt,type=figure}
  \caption[]{Eine Abbildung.}
\end{Example}

Abhilfe schafft ein eigener Stil, der bei solchen Beschriftungen einen anderen
Trenner ohne Zeilenumbruch ausw"ahlt:
\begin{quote}
  |\DeclareCaptionStyle{period-newline}%|\\
  |  [labelsep=period]{labelsep=period-newline}|
\end{quote}
\begin{Example}
  \captionsetup{style=period-newline,labelfont=bf,margin=10pt}
  \captionsetup{aboveskip=0pt,type=figure}
  \ContinuedFloat
  \caption[]{Eine Abbildung.}
\end{Example}
M"ochte man die automatische Zentrierung ebenfalls implementieren, so w"are
\begin{quote}
  |\DeclareCaptionStyle{period-newline}%|\\
  |  [labelsep=period,justification=centering]%|\\
  |  {labelsep=period-newline}|
\end{quote}
eine geeignete Definition:
\begin{Example}
  \captionsetup{style=period-newline2,labelfont=bf,margin=10pt}
  \captionsetup{aboveskip=0pt,type=figure}
  \ContinuedFloat
  \caption[]{Eine Abbildung.}
\end{Example}

Leicht abgewandelt w"urde sich auch bei l"angeren Beschriftungen eine Zentrierung ergeben:
\begin{quote}
  |\DeclareCaptionStyle{period-newline}%|\\
  |  [labelsep=period]%|\\
  |  {labelsep=period-newline,justification=centering}|
\end{quote}
\begin{Example}
  \captionsetup{style=period-newline3,labelfont=bf,margin=10pt}
  \captionsetup{aboveskip=0pt,type=figure}
  \caption[]{\figuretext}
\end{Example}

\bigskip\pagebreak[3]
Ein anderes Beispiel: Die Beschriftungen sollen wie folgt aussehen:
\begin{Example}
  \captionsetup{format=reverse,labelformat=fullparens,labelsep=fill,font=small,labelfont=it}
  \captionsetup{aboveskip=0pt}
  \captionof{figure}[]{\figuretext}
\end{Example}
\pagebreak[2]
Dies lie"se sich z.B. wie folgt realisieren:
\nopagebreak[3]
{\leftmargini=10pt
 \begin{quote}
   |\DeclareCaptionFormat{reverse}{#3#2#1}|\\
   |\DeclareCaptionLabelFormat{fullparens}{(\bothIfFirst{#1}{ }#2)}|\\
   |\DeclareCaptionLabelSeparator{fill}{\hfill}|\\
   |\captionsetup{format=reverse,labelformat=fullparens,|\\
   |              labelsep=fill,font=small,labelfont=it}|
 \end{quote}}

\bigskip\pagebreak[3]
Ein weiteres Beispiel: Der Bezeichner soll in den linken Rand verlagert
werden, so da"s die komplette Absatzbreite der Beschriftung selber zugute kommt:
{\leftmargini=10pt
 \begin{quote}
   |\DeclareCaptionFormat{llap}{\llap{#1#2}#3\par}|\\
   |\captionsetup{format=llap,singlelinecheck=no,labelsep=quad}|
 \end{quote}}
Das Ergebnis w"aren Beschriftungen wie diese:
\begin{Example}
  \captionsetup{format=llap,labelsep=quad,singlelinecheck=no}
  \captionsetup{aboveskip=0pt}
  \captionof{figure}[]{\figuretext}
\end{Example}

% --------------------------------------------------------------------------- %

\pagebreak[4]
\section{Verwendung mit speziellen Dokumentenklassen}

\NEWdescription{v3.0p}
Das \thispackage"=Paket ist auf die Verwendung mit den
Standard"=Dokumentenklassen |article|, |report| und |book| ausgelegt;
ferner funktioniert es mit den Niederl"andischen Klassen |artikel|,
|rapport| und |boek|. Es ist \emph{inkompatibel} mit allen anderen
Dokumentenklassen, es sei denn, sie basieren auf einer der oben genannten.

Im Zweifelsfalle ist von der Verwendung des \thispackage"=Paketes abzuraten.
Man kann versuchen, es trotzdem einzubinden und hoffen, da"s das Dokument
"ubersetzt und sich keine Nebeneffekte einstellen. Ein Nebeneffekt w"are
zum Beispiel die Tatsache, da"s sich alleine durch das Einbinden des
\thispackage"=Paketes ohne Optionen das Aussehen der Bild- oder
Tabellenbeschriftungen "andert. (Ist dies der Fall, mu"s man damit rechnen,
da"s sich die Ausgabe bei der Verwendung von zuk"unftigen Versionen des
\thispackage"=Paketes "andern kann.) Ist dies in Ordnung, so kann man
Einstellungen an den Beschriftungen setzen und die Finger gekreuzt halten.

Die Version \version{3.1} des \thispackage"=Paketes wird an viele
weitere Dokumentenklassen, wie z.B.~die \package{beamer}"=Klasse und
die \KOMAScript"=Klassen, angepasst sein. Die Ver"offentlichung ist
f"ur Sommer 2007 geplant.

% --------------------------------------------------------------------------- %

\pagebreak[3]
\section{Interaktion mit anderen Paketen}
\label{packages}

Das \thispackage"=Paket enth"alt spezielle Anpassungen an andere Pakete, damit
die Beschriftungen dort ebenfalls genauso ausgegeben werden, wie man es mit den oben
genannten Optionen eingestellt hat. Im einzelnen sind dies die folgenden Pakete:

\begin{tabular}{ll}
  |float|        & Erlaubt die Definition eigener gleitenen Umgebungsstile\\
% |hyperref|     & Setzt Hyperlinks\\
% |hypcap|       & Korrigiert die von \package{hyperref} gesetzten Anker bei Beschriftungen\\
  |listings|     & Setzt Quelltexte diverser Programmiersprachen\\
  |longtable|    & Setzt Tabellen, die sich "uber mehrere Seiten erstrecken k"onnen\\
  |rotating|     & Unterst"utzt rotierende Abbildungen und Tabellen\\
  |sidecap|      & Erlaubt das Setzen von Beschriftungen \emph{neben} Abbildungen\\
  |supertabular| & Setzt Tabellen, die sich "uber mehrere Seiten erstrecken k"onnen\\
\end{tabular}

\NEWfeature{v3.0b}
Wird eines dieser Pakete zusammen mit dem \thispackage"=Paket verwendet, steht
einem zus"atzlich die M"oglichkeit bereit, mittels
\begin{quote}|\captionsetup|\oarg{Umgebung}\marg{Optionen}\end{quote}
Optionen festzulegen, die lediglich f"ur diese Umgebung gelten. So bewirkt z.B.
\begin{quote}|\captionsetup[lstlisting]{labelfont=bf}|\quad,\end{quote}
da"s Beschriftungen innerhalb der |lstlisting|"=Umgebung automatisch mit fettem
Bezeichner gesetzt werden.
(Dies funktioniert allerdings nicht mit den |sideways|"=Umgebungen, die vom
\package{rotating}"=Paket angeboten werden.)

Ist die Unterst"utzung eines dieser Pakete im speziellen Falle nicht erw"unscht,
so kann dies durch Angabe der Option
\begin{quote}
  |\usepackage[|\ldots|,|\meta{Paketname}|=no]{caption}|
\end{quote}
erreicht werden, etwa |float=no|, wenn die Unterst"utzung des
\package{float}"=Paketes nicht erw"unscht wird. (Hinweis: Diese Optionen k"onnen
nur innerhalb des |\usepackage|"=Befehls angegeben werden, also insbesondere
\emph{nicht} nachtr"aglich mit |\captionsetup|.)

N"ahere Informationen zu den einzelnen Paketen entnehmen Sie bitte der
dazugeh"origen Anleitung oder dem \LaTeX-Begleiter\cite{companion}.

% --------------------------------------------------------------------------- %

\subsection{Das \package{float}-Paket}
\label{float}

Ein sehr n"utzliches Feature stellt das \package{float}"=Paket\cite{float}
mit dem Platzierungsparameter |[H]| bereit:
Anders als beim Parameter |h|, den \LaTeX\ bereitstellt und der lediglich
eine Empfehlung darstellt, die Abbildung oder Tabelle nach M"oglichkeit
"`hier"' zu setzen, ist das |H| viel kompromi"sloser, denn es erzwingt
das Setzen genau an diesem Ort und nirgendwo anders.

Weiterhin definiert es f"ur gleitende Umgebungen die Stile |plain|,
|plaintop|, |ruled| und |boxed|.
F"ur die vorhandenen Umgebungen |figure| und |table| kann hierbei der Stil
ge"andert werden, ferner k"onnen eigene Umgebungstypen definiert werden,
die ggf.~ein eigenes Verzeichnis bekommen.

Bzgl.~der Abst"ande ist zu beachten, da"s bei Umgebungen des Stils |plain|,
|plaintop| und |boxed| lediglich |\abovecaptionskip| (und kein
|\belowcaptionskip|) zur Anwendung kommt. Ferner wird dieser Abstand vom
\package{float}"=Paket gesetzt und nicht vom \package{caption}"=Paket;
das hat f"ur Sie als Anwender zur Folge, da"s dieser Abstand nicht innerhalb
der Umgebung selbst mit |\captionsetup| ver"andert werden kann, ferner ist
die Option |position=| bei diesen Umgebungen wirkungslos.

Beim Stil |boxed| ist der Abstand mit
\begin{quote}
  |\captionsetup[boxed]{skip=2pt}|
\end{quote}
voreingestellt, bei |plain| und |plaintop| wird die globale Einstellung
verwendet, sofern keine lokale definiert wurde.

Kommt das \package{float}"=Paket zusammen mit dem \thispackage"=Paket zum
Einsatz, so wird automatisch der Beschriftungsstil |ruled| definiert, der das
Aussehen der Beschriftungen innerhalb von Abbildungen des Umgebungsstils
|ruled| regelt:
\begin{quote}
  |\DeclareCaptionStyle{ruled}{labelfont=bf,labelsep=space}|
\end{quote}
F"ur den Anwender bedeutet dies, da"s allgemein get"atigte Einstellungen an den
Beschriftungen hier unwirksam sind; stattdessen werden die Beschriftungen genau
so gesetzt, wie vom \package{float}"=Paket stilistisch vorgegeben, n"amlich so:

\ifx\floatstyle\undefined

\begin{Example}
\hrule height.8pt depth0pt \kern2pt
\vbox{\strut{\bfseries Programm 7.1}
   Das erste Programm. Dies hat nichts mit dem Paket an sich zu tun,
   dient aber als Beispiel. Man beachte den \texttt{ruled} Stil.}
\kern2pt\hrule\kern2pt
\begin{verbatim}
#include <stdio.h>

int main(int argc, char **argv)
{
       for (int i = 0; i < argc; ++i)
               printf("argv[%d] = %s\n", i, argv[i]);
       return 0;
}
\end{verbatim}
\kern2pt\hrule\relax
\end{Example}

\else

\floatstyle{ruled}
\newfloat{Program}{tbp}{lop}[section]
\floatname{Program}{Programm}

\begin{Program}[H]
\begin{verbatim}
#include <stdio.h>

int main(int argc, char **argv)
{
       for (int i = 0; i < argc; ++i)
               printf("argv[%d] = %s\n", i, argv[i]);
       return 0;
}
\end{verbatim}
\caption{Das erste Programm. Dies hat nichts mit dem Paket an sich zu tun,
   dient aber als Beispiel. Man beachte den \texttt{ruled} Stil.}
\end{Program}

\fi

M"ochte man das Aussehen dieser Beschriftungen "andern, ist der Stil |ruled|
mittels
\begin{quote}
  |\DeclareCaptionStyle{ruled}|\marg{Optionen}
\end{quote}
geeignet zu definieren.

Dieser Mechanismus funktioniert auch bei allen anderen Umgebungsstilen,
d.h.~auch bei Umgebungen des Types |plain|, |plaintop| und |boxed| kann ein
geeigneter Beschriftungsstil mit gleichem Namen definiert werden, der dann
automatisch bei gleitenden Umgebungen dieses Types zum Einsatz kommt.

% --------------------------------------------------------------------------- %

\subsection{Das \package{listings}-Paket}
\label{listings}

\NEWdescription{v3.0b}
Das \package{listings}"=Paket\cite{listings} erlaubt die Einbindung von
Quelltexten diverser Programmiersprachen.

\textbf{Achtung:} Die Zusammenarbeit klappt erst ab der Version 1.2 des
\package{listings}"=Paketes. "Altere Versionen verursachen eine Fehlermeldung!

% --------------------------------------------------------------------------- %

\subsection{Das \package{longtable}-Paket}
\label{longtable}

Das \package{longtable}"=Paket\cite{longtable} definiert die Umgebung
|longtable|, die sich wie eine Tabelle anwenden l"a"st, aber im Gegensatz zu
|tabular| Seitenumbr"uche innerhalb der Tabelle gestattet.

% TODO: \DANGER wg. Abstand zur \caption, der f"ur "Uberschriften ausgelegt ist
% => "tableposition=b"
% --------------------------------------------------------------------------- %

\subsection{Das \package{rotating}-Paket}
\label{rotating}

Das \package{rotating}"=Paket\cite{rotating} stellt u.a.~die
gleitenden Umgebungen \texttt{sideways\-figure} und \texttt{sideways\-table}
bereit, die im Gegensatz zu |figure| und |table| um 90 Grad gedreht werden
und immer eine ganze Seite einnehmen.

% --------------------------------------------------------------------------- %

\subsection{Das \package{sidecap}-Paket}
\label{sidecap}

\NEWdescription{v3.0b}
Das \package{sidecap}"=Paket\cite{sidecap} definiert die Umgebungen |SCfigure|
und |SCtable|, die analog zu |figure| und |table| funktionieren, aber
Beschriftungen \emph{neben} der Abbildung oder Tabelle erlauben.

Bei der Verwendung des \package{sidecap}"=Paketes ist zu beachten, da"s eine
dort angegebene Option |raggedright|, |raggedleft| oder |ragged| den Parameter
|justification=| des \thispackage"=Paketes f"ur die betreffenen Umgebungen
"uberschreibt, d.h.~bei Beschriftungen \emph{neben} der Abbildung oder Tabelle
erh"alt die Option des \package{sidecap}"=Paketes den Vorzug.

\DescribeMacro{listof=}
%\NEWfeature{v3.0b}
Ferner liegt es im Design des \package{sidecap}"=Paketes begr"undet,
da"s das Unterdr"ucken des Verzeichniseintrages mit |\caption[]{|\ldots|}|
hier nicht klappt. Als Alternative kann in diesen F"allen die Unterdr"uckung
mittels |\captionsetup{listof=false}| innerhalb der Abbildung oder Tabelle
geschehen.

\ifx\SCfigure\undefined

\begin{Example}
  \newsavebox\scbox
  \begin{lrbox}{\scbox}
    \setlength{\unitlength}{.75cm}%
    \setlength{\fboxsep}{0pt}%
    \fbox{\begin{picture}(4,4)%
      \put(1,3){\circle{1}}%
      \put(3,3){\circle{1}}%
      \put(2,2){\circle{1}}%
      \put(1,1){\circle{1}}%
      \put(3,1){\circle{1}}%
    \end{picture}}%
  \end{lrbox}
  \newlength\scboxwidth
  \setlength\scboxwidth{\wd\scbox}
  \makebox[\linewidth][c]{%
    \parbox[b]{\scboxwidth}{\unhbox\scbox}%
    \hspace\marginparsep
    \parbox[b]{1.5\scboxwidth}{%
      \captionsetup{justification=RaggedRight,labelfont=bf}
      \captionof{figure}[]{Ein kleines Beispiel mit Beschriftung neben der Abbildung.}%
    }%
  }
\end{Example}

\else

\captionsetup{labelfont=bf}
\begin{SCfigure}[1.5][!ht]
  \setlength{\unitlength}{.75cm}%
  \setlength{\fboxsep}{0pt}%
  \fbox{\begin{picture}(4,4)%
    \put(1,3){\circle{1}}%
    \put(3,3){\circle{1}}%
    \put(2,2){\circle{1}}%
    \put(1,1){\circle{1}}%
    \put(3,1){\circle{1}}%
  \end{picture}}%
% \captionsetup{labelfont=bf}
  \caption[]{Ein kleines Beispiel mit Beschriftung neben der Abbildung.}
\end{SCfigure}
\captionsetup{labelfont=default}

\fi

% --------------------------------------------------------------------------- %

\subsection{Das \package{supertabular}-Paket}

Das \package{supertabular}"=Paket\cite{supertabular} definiert, "ahnlich wie
das \package{longtable}"=Paket, eine Umgebung |supertabular|, die sich
ebenfalls wie eine Tabelle anwenden l"a"st, aber im Gegensatz zu |tabular|
Seitenumbr"uche innerhalb der Tabelle gestattet.

Eine ausf"uhrliche Behandlung der Unterschiede zwischen den beiden Paketen
\package{longtable} und \package{supertabular} ist im Buch "`Der \LaTeX-Begleiter"'
\cite{companion} zu finden.

% --------------------------------------------------------------------------- %

\subsection{Bekannte Inkompatibilit"aten}

\NEWdescription{v3.0b}
Die Verwendung des \thispackage"=Paketes in Verbindung mit folgenden Paketen
ist nicht empfehlenswert, da es zu unerw"unschten Seiteneffekten
oder gar Fehlern kommen kann:
\begin{quote}
  \package{ccaption}, \package{ftcap}, \package{hvfloat} und
  \package{nonfloat}
\end{quote}

% --------------------------------------------------------------------------- %

\pagebreak[4]
\section{Kompatibilit"at zu "alteren Versionen}
\label{compatibility}

\subsection{Das \package{caption}-Paket Version $1.x$}

Diese Version des \thispackage"=Paketes ist weitgehend kompatibel zu "alteren
Versionen des Paketes; alte, vorhandene Dokumente sollten sich also in der
Regel ohne Probleme weiterhin "ubersetzen lassen. (Sollten wider Erwarten
Probleme auftauchen, schreiben sie mir bitte eine E-Mail.)

Jedoch ist zu beachten, da"s eine Mischung aus alten Befehlen und neueren
Optionen bzw.~Befehlen zu unerw"unschten Nebeneffekten f"uhren kann.

Hier eine kurze "Ubersicht "uber die alten, "uberholten Optionen und ihre
aktuellen Entsprechungen:

{\small\begin{longtable}{ll}
\package{caption} \version{1.x} & \thispackage\ \version{3.x}\\
\hline
\endhead
|normal|        & |format=plain|\\
|hang|          & |format=hang|\\
|isu|           & |format=hang|\\
|center|        & |justification=centering|\\
|centerlast|    & |justification=centerlast|\\
%|anne|         & |justification=centerlast|\\
|nooneline|     & |singlelinecheck=off|\\
|scriptsize|    & |font=scriptsize|\\
|footnotesize|  & |font=footnotesize|\\
|small|         & |font=small|\\
|normalsize|    & |font=normalsize|\\
|large|         & |font=large|\\
|Large|         & |font=Large|\\
|up|            & |labelfont=up|\\
|it|            & |labelfont=it|\\
|sl|            & |labelfont=sl|\\
|sc|            & |labelfont=sc|\\
|md|            & |labelfont=md|\\
|bf|            & |labelfont=bf|\\
|rm|            & |labelfont=rm|\\
|sf|            & |labelfont=sf|\\
|tt|            & |labelfont=tt|\\
\end{longtable}}

Neben den Optionen zum Einstellen des Zeichensatzes gab es auch die Befehle
|\captionsize| bzw. |\captionfont| und |\captionlabelfont|, die direkt
mittels |\renewcommand| ver"andert werden konnten. Dieser Mechanismus
wurde durch die Anweisungen
\begin{quote}
  |\DeclareCaptionFont{|\ldots|}{|\ldots|}|\qquad und\\
  |\captionsetup{font=|\ldots|,labelfont=|\ldots|}|
\end{quote}
ersetzt. \SeeUserDefined

Das Setzen eines Randes geschah in \version{1.x} mittels
\begin{quote}
  |\setlength{\captionmargin}{|\ldots|}|\quad.
\end{quote}
Dies wurde durch
\begin{quote}
  |\captionsetup{margin=|\ldots|}|
\end{quote}
ersetzt. \See{\Section{margins}{R"ander und Abs"atze}}

Zum Beispiel w"urde
\begin{quote}
|\usepackage[hang,bf]{caption}|\\
|\renewcommand\captionfont{\small\sffamily}|\\
|\setlength\captionmargin{10pt}|
\end{quote}
in aktueller Notation
\begin{quote}
|\usepackage[format=hang,labelfont=bf,font={small,sf},|\\
|            margin=10pt]{caption}|
\end{quote}
bzw.
\begin{quote}
|\usepackage{caption}|\\
|\captionsetup{format=hang,labelfont=bf,font={small,sf},|\\
|              margin=10pt}|
\end{quote}
hei"sen.

Die etwas exotische Option |ruled|, die eine partielle Anwendung der
eingestellten Parameter bei gleitenden Umgebungen des Typs |ruled|
aktivierte, wird ebenfalls emuliert, hat aber keine direkte
Entsprechung in dieser Version des \thispackage"=Paketes.
M"ochte man gezielt das Aussehen der Abbildungen des Stils |ruled|,
der durch das \package{float}"=Paket zur Verf"ugung gestellt wird,
ver"andern, so ist dies nun durch
\begin{quote}
  |\DeclareCaptionStyle{ruled}{|\ldots|}|
\end{quote}
bzw.
\begin{quote}
  |\captionsetup[ruled]{|\ldots|}|
\end{quote}
m"oglich. \SeeUserDefined[ und \Section*{misc}{N"utzliches} sowie
                          \Section*{float}{Das \package{float}-Paket}]

\subsection{Das \package{caption2}-Paket Version $2.x$}

Die Pakete \package{caption} und seine experimentelle, nun veraltete
Variante \package{caption2} sind vom internen Konzept
her zu unterschiedlich, um hier eine vollst"andige Kompatibilit"at
gew"ahrleisten zu k"onnen.
Daher liegt diesem Paket weiterhin die Datei |caption2.sty| bei, so da"s
"altere Dokumente, die das \package{caption2}"=Paket verwenden, weiterhin
"ubersetzt werden k"onnen.

Neue Dokumente sollten jedoch auf dem aktuellen \thispackage"=Paket
aufgesetzt werden. In den meisten F"allen ist es ausreichend, einfach
ggf.~die Anweisung
\begin{quote}
  |\usepackage[...]{caption2}|
\end{quote}
durch
\begin{quote}
  |\usepackage[...]{caption}|
\end{quote}
zu ersetzen. Einige Optionen und Befehle werden jedoch nicht emuliert,
so da"s sie anschlie"send Fehlermeldungen erhalten k"onnen.
Die folgenden Abs"atze werden Ihnen jedoch bei der Umsetzung dieser
Optionen und Befehle helfen. Sollten dar"uberhinaus noch Fragen oder
Probleme auftreten, so z"ogern Sie bitte nicht, mich diesbez"uglich
per E-Mail zu kontaktieren.

Zus"atzlich zu den bereits im vorherigen Abschnitt vorgestellten Optionen
werden auch folgende emuliert:

{\small\begin{longtable}{ll}
\package{caption2} \version{2.x} & \thispackage\ \version{3.x}\\
\hline
\endhead
|flushleft|   & |justification=raggedright|\\
|flushright|  & |justification=raggedleft|\\
|oneline|     & |singlelinecheck=on|\\
\end{longtable}}

Das Setzen eines Randes geschah in \version{2.x} mittels
\begin{quote}\leavevmode\hbox{%
  |\setcaptionmargin{|\ldots|}| bzw.
  |\setcaptionwidth{|\ldots|}|\quad.
}\end{quote}
Dies wurde durch
\begin{quote}\leavevmode\hbox{%
  |\captionsetup{margin=|\ldots|}| bzw.
  |\captionsetup{width=|\ldots|}|
}\end{quote}
ersetzt. \See{\Section{margins}{R"ander und Abs"atze}}

Das Setzen des Einzuges wurde in \version{2.x} mit
\begin{quote}
  |\captionstyle{indent}|\\
  |\setlength\captionindent{|\ldots|}|
\end{quote}
erledigt, dies geschieht nun mit
\begin{quote}
  |\captionsetup{format=plain,indention=|\ldots|}|\quad.
\end{quote}

Die Sonderbehandlung von einzeiligen Beschriftungen lie"s sich in
\version{2.x} mit |\oneline|\-|captions|\-|false| aus-
bzw. |\oneline|\-|captions|\-|true| wieder einschalten. Dies wurde durch
|\captionsetup{|\discretionary{}{}{}|singlelinecheck=|\discretionary{}{}{}|off}|
bzw.
|\captionsetup{|\discretionary{}{}{}|singlelinecheck=|\discretionary{}{}{}|on}|
ersetzt. \See{\Section{justification}{Textausrichtung}}

Die Befehle
\begin{quote}
  |\captionlabeldelim|, |\captionlabelsep|, |\captionlabelfalse|,
  |\captionstyle|, |\defcaptionstyle|, |\newcaptionstyle| und |\renewcaptionstyle|
\end{quote}
haben keine direkte Entsprechnung und werden daher durch diese
Version des \thispackage"=Paketes auch nicht emuliert.
Sie f"uhren also bei der Verwendung %mit diesem \thispackage"=Paket
zu Fehlermeldungen und m"ussen daher zwingend umgesetzt werden.
Die Umsetzung ist von Fall zu Fall verschieden, lesen Sie sich daher bitte
diese Anleitung gr"undlich durch und suchen Sie sich die Optionen bzw.~Befehle
als Ersatz heraus, die Ihren W"unschen entsprechen.
\iffalse
Als kleine Hilfestellung hier die Beispiele aus der alten Anleitung zum
\package{caption2}"=Paket und deren Umsetzung:

\newenvironment{OldNew}%
  {\begin{minipage}\linewidth
   \def\Old{Alt:\begin{quote}}%
   \def\New{\end{quote}Neu:\begin{quote}}%
   \def\Or{\end{quote}\centerline{-- oder --}\begin{quote}}%
  }%
  {\end{quote}\end{minipage}}

\begin{OldNew}
\Old
  |\captionstyle{center}|
\New
  |\captionsetup{justification=centering}|
\end{OldNew}

\hrule

\begin{OldNew}
\Old
  |\captionstyle{indent}|\\
  |\setlength{\captionindent}{1cm}|
\New
  |\captionsetup{format=plain,indention=1cm}|
\end{OldNew}

\hrule

\begin{OldNew}
\Old
  |\renewcommand\captionfont{\small}|\\
  |\renewcommand\captionlabelfont{\itshape}|
\New
  |\captionsetup{font=small,labelfont=it}|
\end{OldNew}

\hrule

\begin{OldNew}
\Old
  |\renewcommand\captionfont{\small\itshape}|\\
  |\renewcommand\captionlabelfont{\upshape}|
\New
  |\captionsetup{font=small,textfont=it}|
\end{OldNew}

\hrule

\begin{OldNew}
\Old
  |\setcaptionwidth{.5\textwidth}|
\New
  |\captionsetup{width=.5\textwidth}|
\end{OldNew}

\hrule

\begin{OldNew}
\Old
  |\setcaptionmargin{.25\textwidth}|
\New
  |\captionsetup{margin=.25\textwidth}|
\end{OldNew}

\hrule

\begin{OldNew}
\Old
  |\newcaptionstyle{absatz}{\captionlabel: \captiontext\par}|\\
  |\captionstyle{absatz}|
\New
  |\DeclareCaptionFormat{absatz}{#1: #3\par}|\\
  |\captionsetup{format=absatz,singlelinecheck=off}|
\Or
  |\captionsetup{format=plain,singlelinecheck=off}|
\end{OldNew}

\hrule

\begin{OldNew}
\Old
  |\newcaptionstyle{fancy}{\textsf{\captionlabel}\\\captiontext\par}|\\
  |\captionstyle{fancy}|
\New
  |\DeclareCaptionFormat{fancy}{\textsf{#1}\\#3\par}|\\
  |\captionsetup{format=fancy,singlelinecheck=off}|
\Or
  |\captionsetup{format=plain,labelfont=sf,labelsep=newline}|
\end{OldNew}

\hrule

\begin{OldNew}
\Old
  |\newcaptionstyle{fancy2}{\captiontext\hfill\textit{(\captionlabel)}}|\\
  |\captionstyle{fancy2}|
\New
  |\DeclareCaptionFormat{fancy2}{#3\hfill\textit{(#1)}}|\\
  |\captionsetup{format=fancy2,singlelinecheck=off}|
\end{OldNew}

\hrule

\begin{OldNew}
\Old
  |\newcaptionstyle{mystyle}{%|\\
  |  \normalcaptionparams|\\
  |  \renewcommand\captionlabelfont{\bfseries}%|\\
  |  \renewcommand\captionlabeldelim{.}%|\\
  |  \onelinecaptionsfalse|\\
  |  \usecaptionstyle{centerlast}}|\\
  |\captionstyle{mystyle}|
\New
  |\DeclareCaptionStyle{mystyle}{labelfont=bf,labelsep=period,justification=centerlast}|\\
  |\captionsetup{style=mystyle}|
\end{OldNew}

\hrule

\begin{OldNew}
\Old
  |\newcaptionstyle{hangandleft}{%|\\
  |  \let\oldcaptiontext\captiontext|\\
  |  \def\captiontext{\raggedright\oldcaptiontext}%|\\
  |  \usecaptionstyle{hang}}|\\
  |\captionstyle{hangandleft}|
\New
  |\captionsetup{format=hang,justification=raggedright}|
\end{OldNew}

\hrule

\begin{OldNew}
\Old
  |\newcaptionstyle{fancy}{%|\\
  |  \usecaptionmargin\captionfont|\\
  |  \onelinecaption|\\
  |    {{\captionlabelfont\captionlabel\captionlabeldelim}%|\\
  |     \captionlabelsep\captiontext}%|\\
  |    {{\centering\captionlabelfont\captionlabel\par}%|\\
  |      \centerlast\captiontext\par}}|\\
  |\captionstyle{fancy}|
\New
  |\DeclareCaptionFormat{fancy}{\centering#1\par\centerlast#3\par}|\\
  |\DeclareCaptionStyle{fancy}|\\
  |  [format=plain,justification=centering]|\\
  |  {format=fancy}|\\
  |\captionsetup{style=fancy}|
\Or
  |\DeclareCaptionFormat{fancy}{#1\par#3\par}|\\
  |\DeclareCaptionStyle{fancy}|\\
  |  [format=plain,justification=centering]|\\
  |  {format=fancy,justification=centerlast}|\\
  |\captionsetup{style=fancy}|
\end{OldNew}

\hrule

\begin{OldNew}
\Old
  |\renewcaptionstyle{longtable}{\usecaptionstyle{normal}}|
\New
  |\captionsetup[longtable]{format=plain}|
\end{OldNew}
\fi

Ebenfalls keine Entsprechung hat die \version{2.x}"=Option |ignoreLTcapwidth|.
Deren Verwendung kann in der Regel einfach entfallen, da das
\thispackage"=Paket den Wert von |\LTcapwidth| sowieso nicht beachtet,
solange er nicht explizit auf einen anderen Wert als den Standardwert
gesetzt wird.
\See{\Section{longtable}{Das \package{longtable}"=Paket}}

% --------------------------------------------------------------------------- %

%\pagebreak[4]
\section{Weiterf"uhrende Dokumente}

Folgende Dokumente m"ochte ich an dieser Stelle jedem ans Herz legen:

\begin{itemize}
\item
  Die DANTE-FAQ:\nopagebreak
  \begin{quote}
    \url{http://www.dante.de/faq/de-tex-faq/}
  \end{quote}

\item
  \emph{"`Gleitobjekte -- die richtige Schmierung"'} von Axel Reichert
  erl"autert den Umgang mit gleitenden Umgebungen und ist hier im Netz
  zu finden:\nopagebreak
  \begin{quote}
    \url{ftp://ftp.dante.de/pub/tex/info/german/gleitobjekte/}
  \end{quote}

\item
  \textsf{epslatex} von Keith Reckdahl enth"alt viele n"utzliche Tips im
  Zusammenhang mit der Einbindung von Graphiken in \LaTeXe.
  Das Dokument ist unter\nopagebreak
  \begin{quote}
    \url{ftp://ftp.dante.de/pub/tex/info/epslatex/}
  \end{quote}
  zu finden.
\end{itemize}

% --------------------------------------------------------------------------- %

%\pagebreak[3]
\section{Danksagungen}

Von ganzem Herzen danke ich Katja Melzner,
Steven D. Cochran, Frank Mittelbach,
David Carlisle, Carsten Heinz, Olga Lapko und Keith Reckdahl.

Weiterhin m"ochte ich mich herzlich bei
Harald Harders,
Peter L\"offler,
Peng Yu,
Alexander Zimmermann,
Matthias Pospiech,
J\"urgen Wieferink,
Christoph Bartoschek,
Uwe St\"ohr,
Ralf Stubner,
Geoff Vallis,
Florian Keiler,
J"urgen G"obel,
Uwe Siart,
Sang-Heon Shim,
Henrik Lundell,
David Byers,
William Asquith
und
Prof.~Dr.~Dirk Hoffmann
f"ur ihre Hilfe beim stetigen Verbessern dieses Paketes bedanken.

% --------------------------------------------------------------------------- %

\pagebreak[4]
\begin{thebibliography}{9}
  \bibitem{companion}
  Frank Mittelbach and Michel Goossens:
  \newblock {\em The {\LaTeX} Companion (2nd.~Ed.)},
  \newblock Addison-Wesley, 2004.

  \bibitem{float}
  Anselm Lingnau:
  \emph{An Improved Environment for Floats},
  2001/11/08

  \bibitem{floatrow}
  Olga Lapko:
  \emph{The floatrow package documentation},
  2005/05/22

  \bibitem{hyperref}
  Sebastian Rahtz \& Heiko Oberdiek:
  \emph{Hypertext marks in \LaTeX},
  2007/01/25

  \bibitem{hypcap}
  Heiko Oberdiek:
  \emph{The hypcap package -- Adjusting anchors of captions}
  2007/02/19

  \bibitem{listings}
  Carsten Heinz:
  \emph{The Listings Package},
  2004/02/13

  \bibitem{longtable}
  David Carlisle:
  \emph{The longtable package},
  2000/10/22

  \bibitem{rotating}
  Sebastian Rahtz and Leonor Barroca:
  \emph{A style option for rotated objects in \LaTeX},
  1997/09/26

  \bibitem{sidecap}
  Rolf Niepraschk und Hubert G"a"slein:
  \emph{The sidecap package},
  2003/06/06

  \bibitem{subfig}
  Steven D. Cochran:
  \emph{The subfig package},
  2005/07/05

  \bibitem{supertabular}
  Johannes Braams und Theo Jurriens:
  \emph{The supertabular environment},
  2002/07/19
\end{thebibliography}

\end{document}
