# Supplementary material for: Operation of a Microfabricated Planar Ion-Trap for Studies of a Yb$^+$-Rb Hybrid Quantum System
Source: arXiv:1811.07670 source file (2019-03-19)
Supplement: Supplementary file 4 [file test3.tex]

%% test3.tex
%%
%% This is file `test3.tex', one of a set of several test/example files
%% in the `subfig' package.
%%
%% Copyright © 2003, 2004, 2005 Steven Douglas Cochran.
%% 
%% This work (the subfig package) may be distributed and/or modified 
%% under the conditions of the LaTeX Project Public License, either 
%% version 1.3 of this license or (at your option) any later version.
%% The latest version of this license is in
%%   http://www.latex-project.org/lppl.txt
%% and version 1.3 or later is part of all distributions of LaTeX
%% version 2003/12/01 or later.
%%
%% This work has the LPPL maintenance status "author-maintained".
%% 
%% This Current Maintainer of this work is Steven Douglas Cochran.
%%
%% This work consists of all files listed under "MANIFEST" in the
%% README file distributed with the subfig package.

\documentclass{article}

\usepackage{fullpage}
\usepackage[config=altsf]{subfig}
\usepackage{booktabs}

\newdimen\testtemp
\newcommand{\ru}[1]{%
  \testtemp #1%
  \advance\testtemp .5pt%
  \divide\testtemp 2%
  \hbox to \testtemp{\leaders\hbox to 1mm{%
    \vrule height1mm depth0pt width.25pt\hfil}\hfil}%
  \hbox to 0pt{\hss\vrule height3mm depth0pt width.25pt\hss}%
  \hbox to \testtemp{\leaders\hbox to 1mm{%
    \hfil\vrule height1mm depth0pt width.25pt}\hfil}}

\makeatletter
  \renewcommand\abstract[1]{%
    \def\@abstract{%
      \centerline{{\large\bf Abstract}}
      \noindent
      #1}}
  \renewcommand\@maketitle{%
    \newpage
    \null\vfil
    \vskip 60\p@
    \begin{center}%
      {\LARGE \@title \par}%
      \vskip 3em%
      {\large
       \lineskip .75em%
       \begin{tabular}[t]{c}%
         \@author
       \end{tabular}\par}%
      \vskip 1.5em%
      {\large \@date \par}% 
    \end{center}%
    \vskip 2.5em%
    \@abstract
    \vfil\null}%
\makeatother

\def\textfraction{.1}
\fboxsep=-\fboxrule
\newcommand{\figbox}[1]{%
  \fbox{%
    \vbox to 1in{%
      \vfil
      \hbox to 2in{%
        \parbox{2in}{%
          \centering
          #1}}%
      \vfil
      \vbox to 0pt{%
        \vss
        \hbox to 2in{%
          \hfil
          \ru{1.1in}%
          \hfil}}}}}

\begin{document}

\title{Subfig Package Test Program Three}
\author{Steven Douglas Cochran\\
        Digital Mapping Laboratory\\
        School of Computer Science\\
        Carnegie-Mellon University\\
        5000 Forbes Avenue\\
        Pittsburgh, PA 15213-3890\\
        USA}
\date{21 December 2003}
\abstract{%
This test checks three things:
\begin{enumerate}
  \item spacing is reduced at the start of a minipage or between
        horizontal layers of subfloats;
  \item extra blank spaces; and,
  \item together with initialization options, that the subfig.cfg
        file provides approximate compatibility with the old
        {\bf subfigure} package.
\end{enumerate}}
\maketitle
\clearpage

\setcounter{lofdepth}{2}
\listoffigures
\newpage

\section{Reference Test}

\begin{figure}%
  \centering
  \subfigure{%
    \label{fig:A}%
    \figbox{SUBFIGURE ONE:\\
            (no opt)}}
  \quad
  \subfigure[]{%
    \label{fig:B}%
    \figbox{SUBFIGURE TWO:\\
            (empty opt)}}\\
%
  \subfigure[Subfigure Three.]{%
    \label{fig:C}%
    \figbox{SUBFIGURE THREE:\\
            (opt)}}
  \quad
  \subfigure[][Subfigure Four.]{%
    \label{fig:D}%
    \figbox{SUBFIGURE FOUR:\\
            (empty opt and opt)}}
  \quad
  \subfigure[][]{%
    \label{fig:E}%
    \figbox{SUBFIGURE FIVE:\\
            (both empty opt)}}\\
%
  \subfigure[The Sixth Subfigure.][Subfigure Six.]{%
    \label{fig:F}%
    \figbox{SUBFIGURE SIX:\\
            (both opt)}}
  \quad
  \subfigure[The Seventh Subfigure][]{%
    \label{fig:G}%
    \figbox{SUBFIGURE SEVEN:\\
            (opt and empty opt)}}
%
  \caption{Optional argument test.}%
  \label{fig:main}%
\end{figure}

The figure~\ref{fig:main} on page~\pageref{fig:main} is composed
of the seven subfigures~\subref{fig:A} (aka: \ref{fig:A}),
\subref{fig:B} (aka: \ref{fig:B}), \subref{fig:C} (aka: \ref{fig:C}),
\subref{fig:D} (aka: \ref{fig:D}), \subref{fig:E} (aka: \ref{fig:E}),
\subref{fig:F} (aka: \ref{fig:F}), and \subref{fig:G} (aka:
\ref{fig:G}).

Note that the captions are correctly handled on the List-of-Figures
page and under the subfigures according to the form of the subfigure
command (see Table~\ref{tab:calling}).

\begin{table}[b]
  \centering
  \caption{{\tt ${\tt\backslash}$subfigure} calling arguments.}
  \label{tab:calling}
  \begin{tabular}{llc}                                      \\ \toprule
    {\bf Subfigure Command}
                      & {\bf LoF/LoT}
                            & \multicolumn{1}{l}{\bf Subfigure Caption}
                                                            \\ \midrule
    \verb/\subfigure/\{\dots fig\dots\}
                      &     &                               \\
    \verb/\subfigure/[~]\{\dots fig\dots\}
                      & (b)\ \ . . . . . . . . . .  
                            & (b)                           \\
    \verb/\subfigure/[Subcaption.]\{\dots fig\dots\}
                      & (c) Subcaption. . . .
                            & (c) Subcaption.               \\
    \verb/\subfigure/[\space][Subcaption.]\{\dots fig\dots\}
                      &     & (d) Subcaption.               \\
    \verb/\subfigure/[\space][\space]\{\dots fig\dots\}
                      &     & (e)                           \\
    \verb/\subfigure/[List\_entry.][Subcaption.]\{\dots fig\dots\}
                      & (f) List\_entry. . . .
                            & (f) Subcaption.               \\
    \verb/\subfigure/[List\_entry.][~]\{\dots fig\dots\}
                      & (g) List\_entry. . . .
                            & (g)                           \\ \bottomrule
  \end{tabular}
\end{table}

\enlargethispage{12pt}
\section{Centering Test}

Note that figures~\ref{fig:B}, \ref{fig:E} and \ref{fig:G} are centered.
This means that \verb|\subfigcapskip| has been set to zero and is not
offsetting the simple label to the left.  Also the remaining captioned
subfigures (figures~\ref{fig:C}, \ref{fig:D}, and \ref{fig:F}) should
have centered labels.


\end{document}
